# Supplementary material for: AttWalk: Attentive Cross-Walks for Deep Mesh Analysis
Source: arXiv:2104.11571 source file (2021-04-23)
Supplement: Supplementary file 1 [file supplemental.tex]

\section{Introduction}

% ========== SHREC '16 retrieval table ================  %
\begin{table*}[t]
\begin{center}
\begin{tabular}{ |l c c c c c c|c c c c c|}
\hline
 & & \multicolumn{5}{c|}{microAll} & \multicolumn{5}{c|}{macroAll} \\
% \cline{2-11}
\hline
Method & Input & P@N & R@N & F1@N & mAP & NDCG & P@N & R@N & F1@N & mAP & NDCG \\
\hline
Ours by prediction  & Mesh & 52.9 & 91.7 & 60.6 & \bf{81.1} & \bf{86.6}
              & 15.4 & 88.6 & 21.2 & \bf{65.5} & \bf{68.2}\\
Ours by $f_a$  & Mesh & 52.0 & 90.3 & 59.6 & 78.8 & 85.6
              & 15.2 & 88.0 & 20.9 & 60.9 & 65.1 \\
% MeshWalker \cite{lahav2020meshwalker} (prediction)  & Mesh & 52.8 & 91.1 & 60.5 & 80.6 & 86.0 
%                                               & 15.3 & 86.7 & 21.0 & 64.3 & 67.1 \\
ViewGCN~\cite{wei2020view}      & multi-views & 81.8 & 80.9 & \bf{80.6} & 78.4 & 85.2
                                              & \bf{62.9} & 65.2 & \bf{61.1} & 60.2 & 66.5 \\
GIFT~\cite{bai2016gift}         & multi-views & 70.6 & 69.5 & 68.9 & 64.0 & 76.5 
                                              & 44.4 & 53.1 & 45.4 & 44.7 & 54.8 \\
MVCNN~\cite{su2015multi}        & multi-views & 77.0 & 77.0 & 76.4 & 73.5 & 81.5
                                              & 57.1 & 62.5 & 57.5 & 56.6 & 64.0 \\
RotationNet~\cite{kanezaki2018rotationnet} &  multi-views & 81.0 & 80.1 & 79.8 & 77.2 & 86.5
                                                          & 60.2 & 63.9 & 59.0 & 58.3 & 65.6 \\
                                           
% Following paper published with old SHREC2017 evaluation code, wrong results. no released code and no released info so cannot re-run with corrected code
% DeepGM \cite{luciano2018geodesic}   & 78.4 & 73.2 & 69.6 & 93.6 & 96.5 
%                & 85.4 & 45.9 & 52.3 & 92.2 & 95.8 \\
\hline
\end{tabular}
\end{center}
\caption{\ran{Shape retrieval results on ShapeNet Core55 normal test set.} \ayellet{put the full table in the supplemental, keep only MAP\\NDCG?} \ayellet{mesh-walker with the same number of walks in all tables}}
\label{tab:shapenet_retrieval}
\end{table*}

% ==========  Attention on Modelnet40 where we fix prediction of original MeshWalker ======= #
% Qualitative examples - attention fix prediction
\ran{Cases our attention predict correctly where without it it fails}
\begin{figure*}
\begin{subfigure}{.25\textwidth}
  \centering
  \includegraphics[width=.9\linewidth]{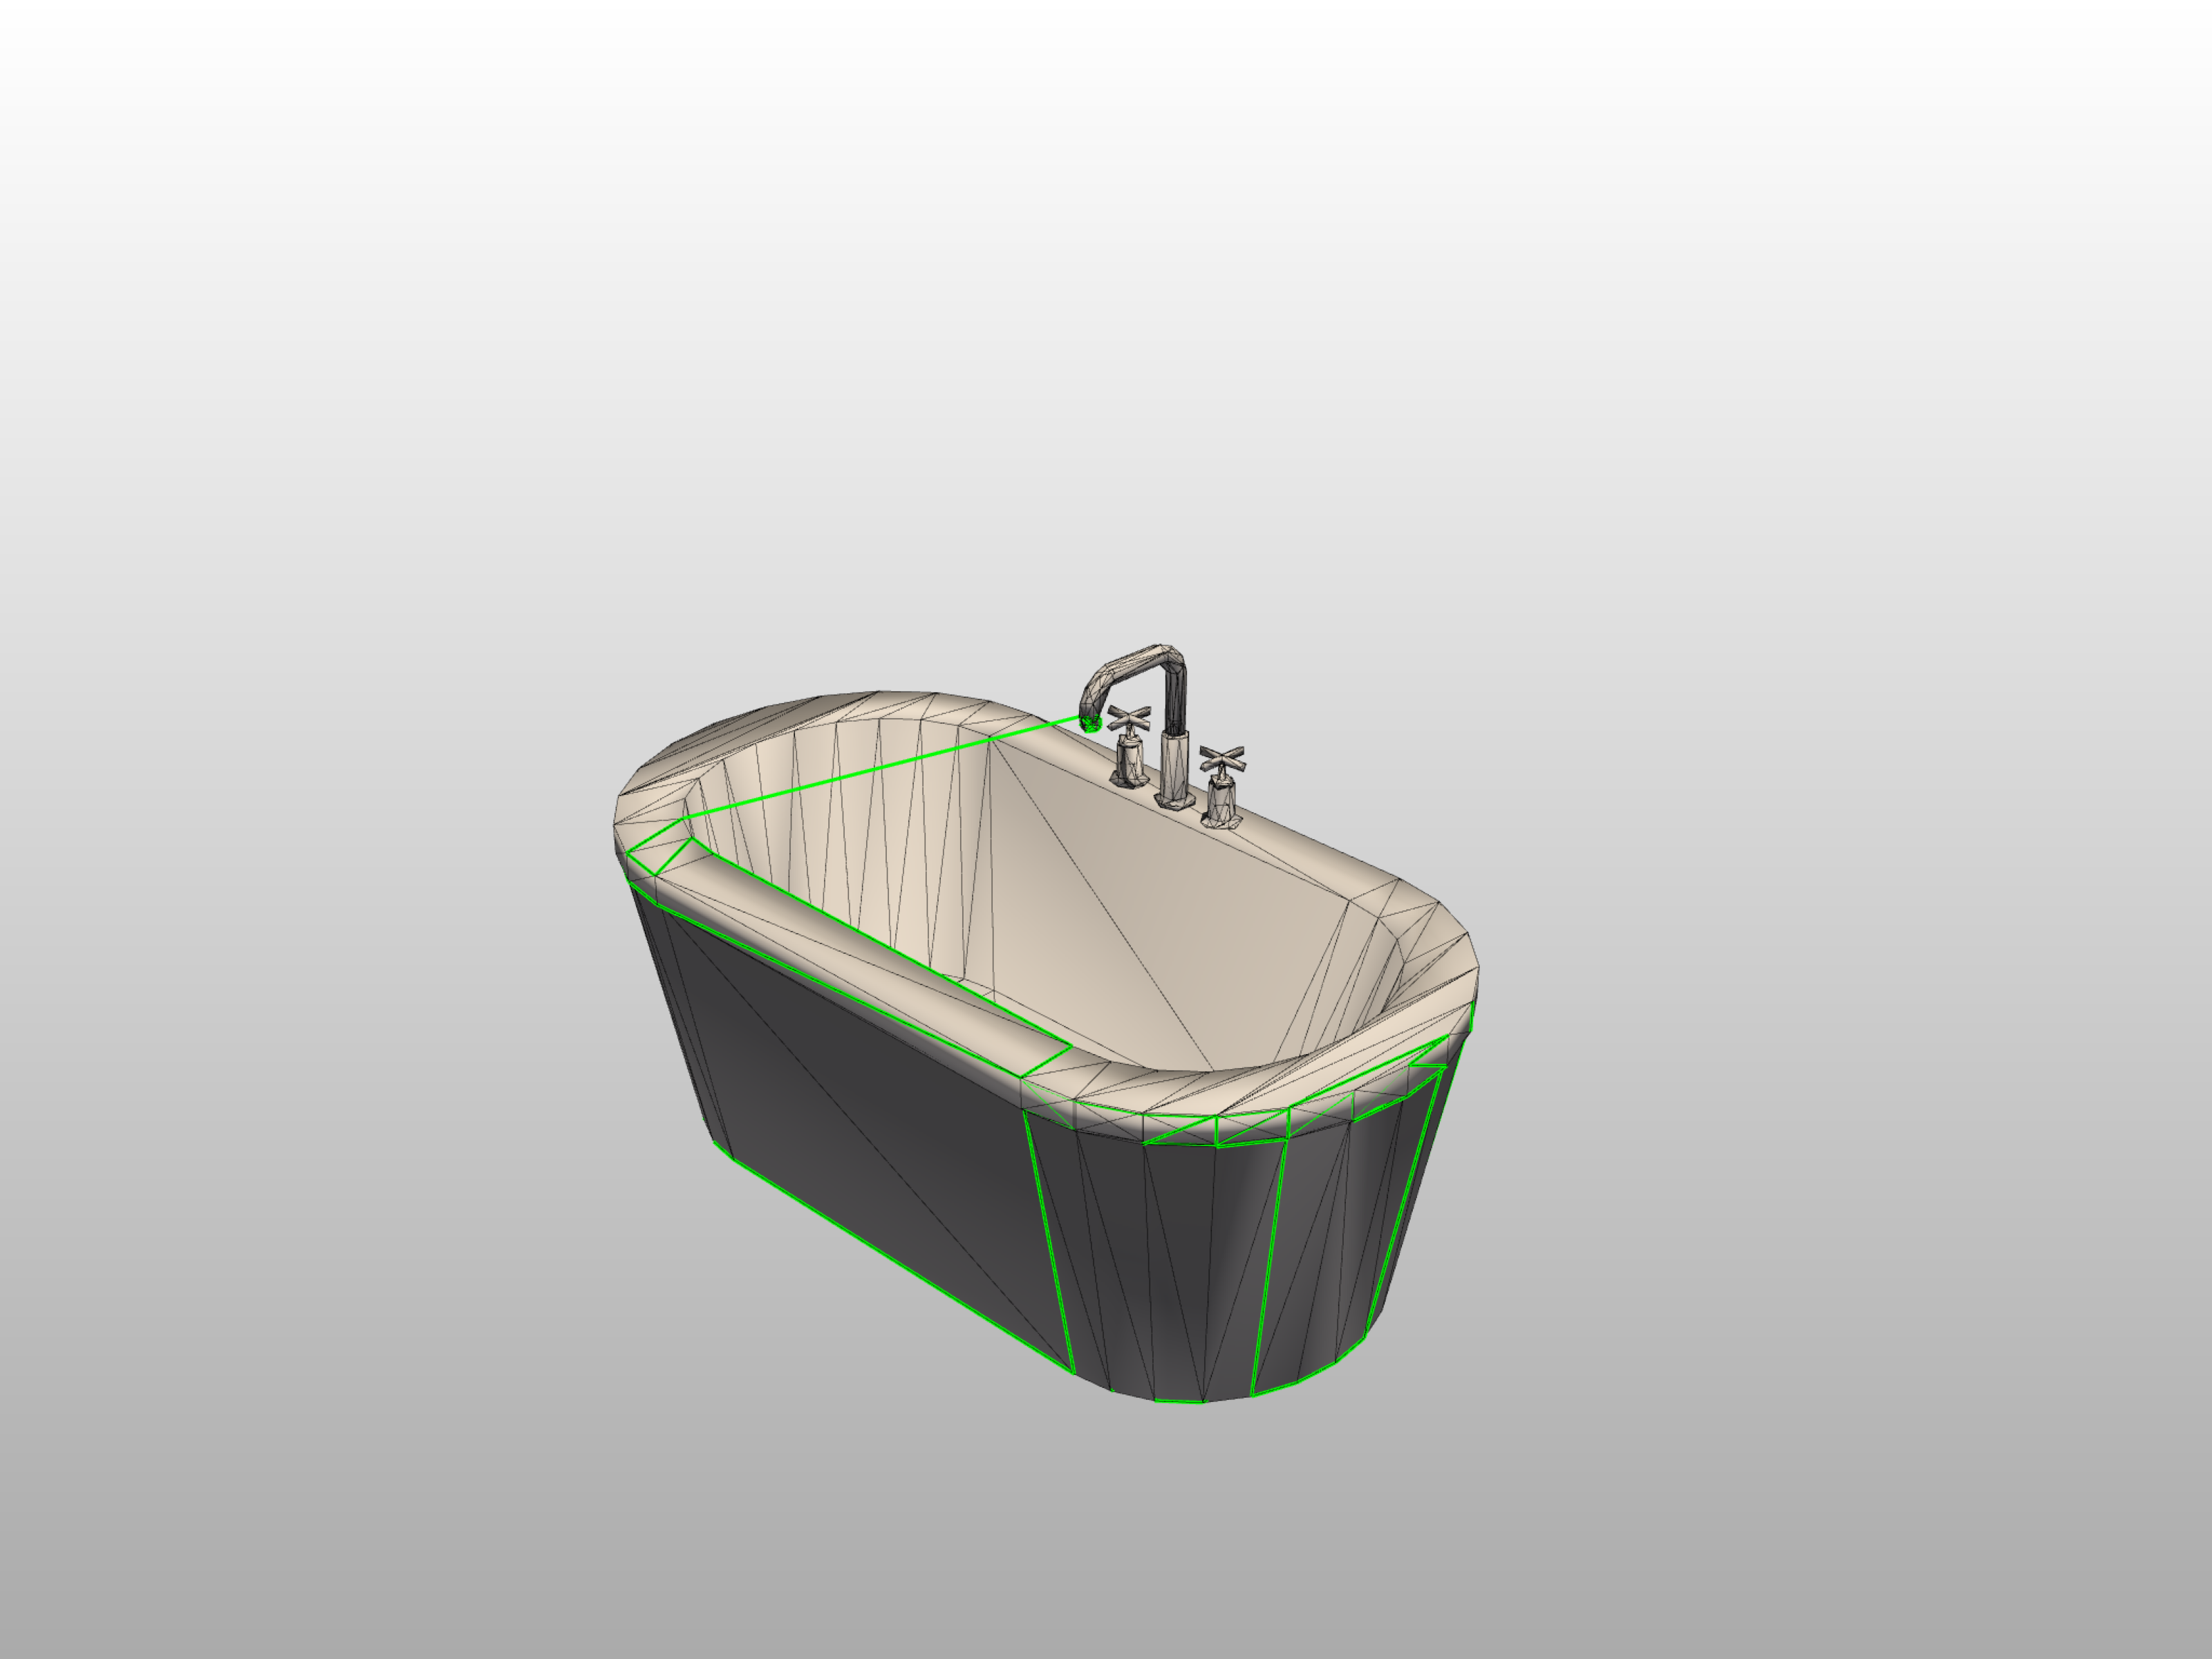}
  \caption{25\%}
  \label{fig:attn_bathtub_1st}
\end{subfigure}%
\begin{subfigure}{.25\textwidth}
  \centering
  \includegraphics[width=.9\linewidth]{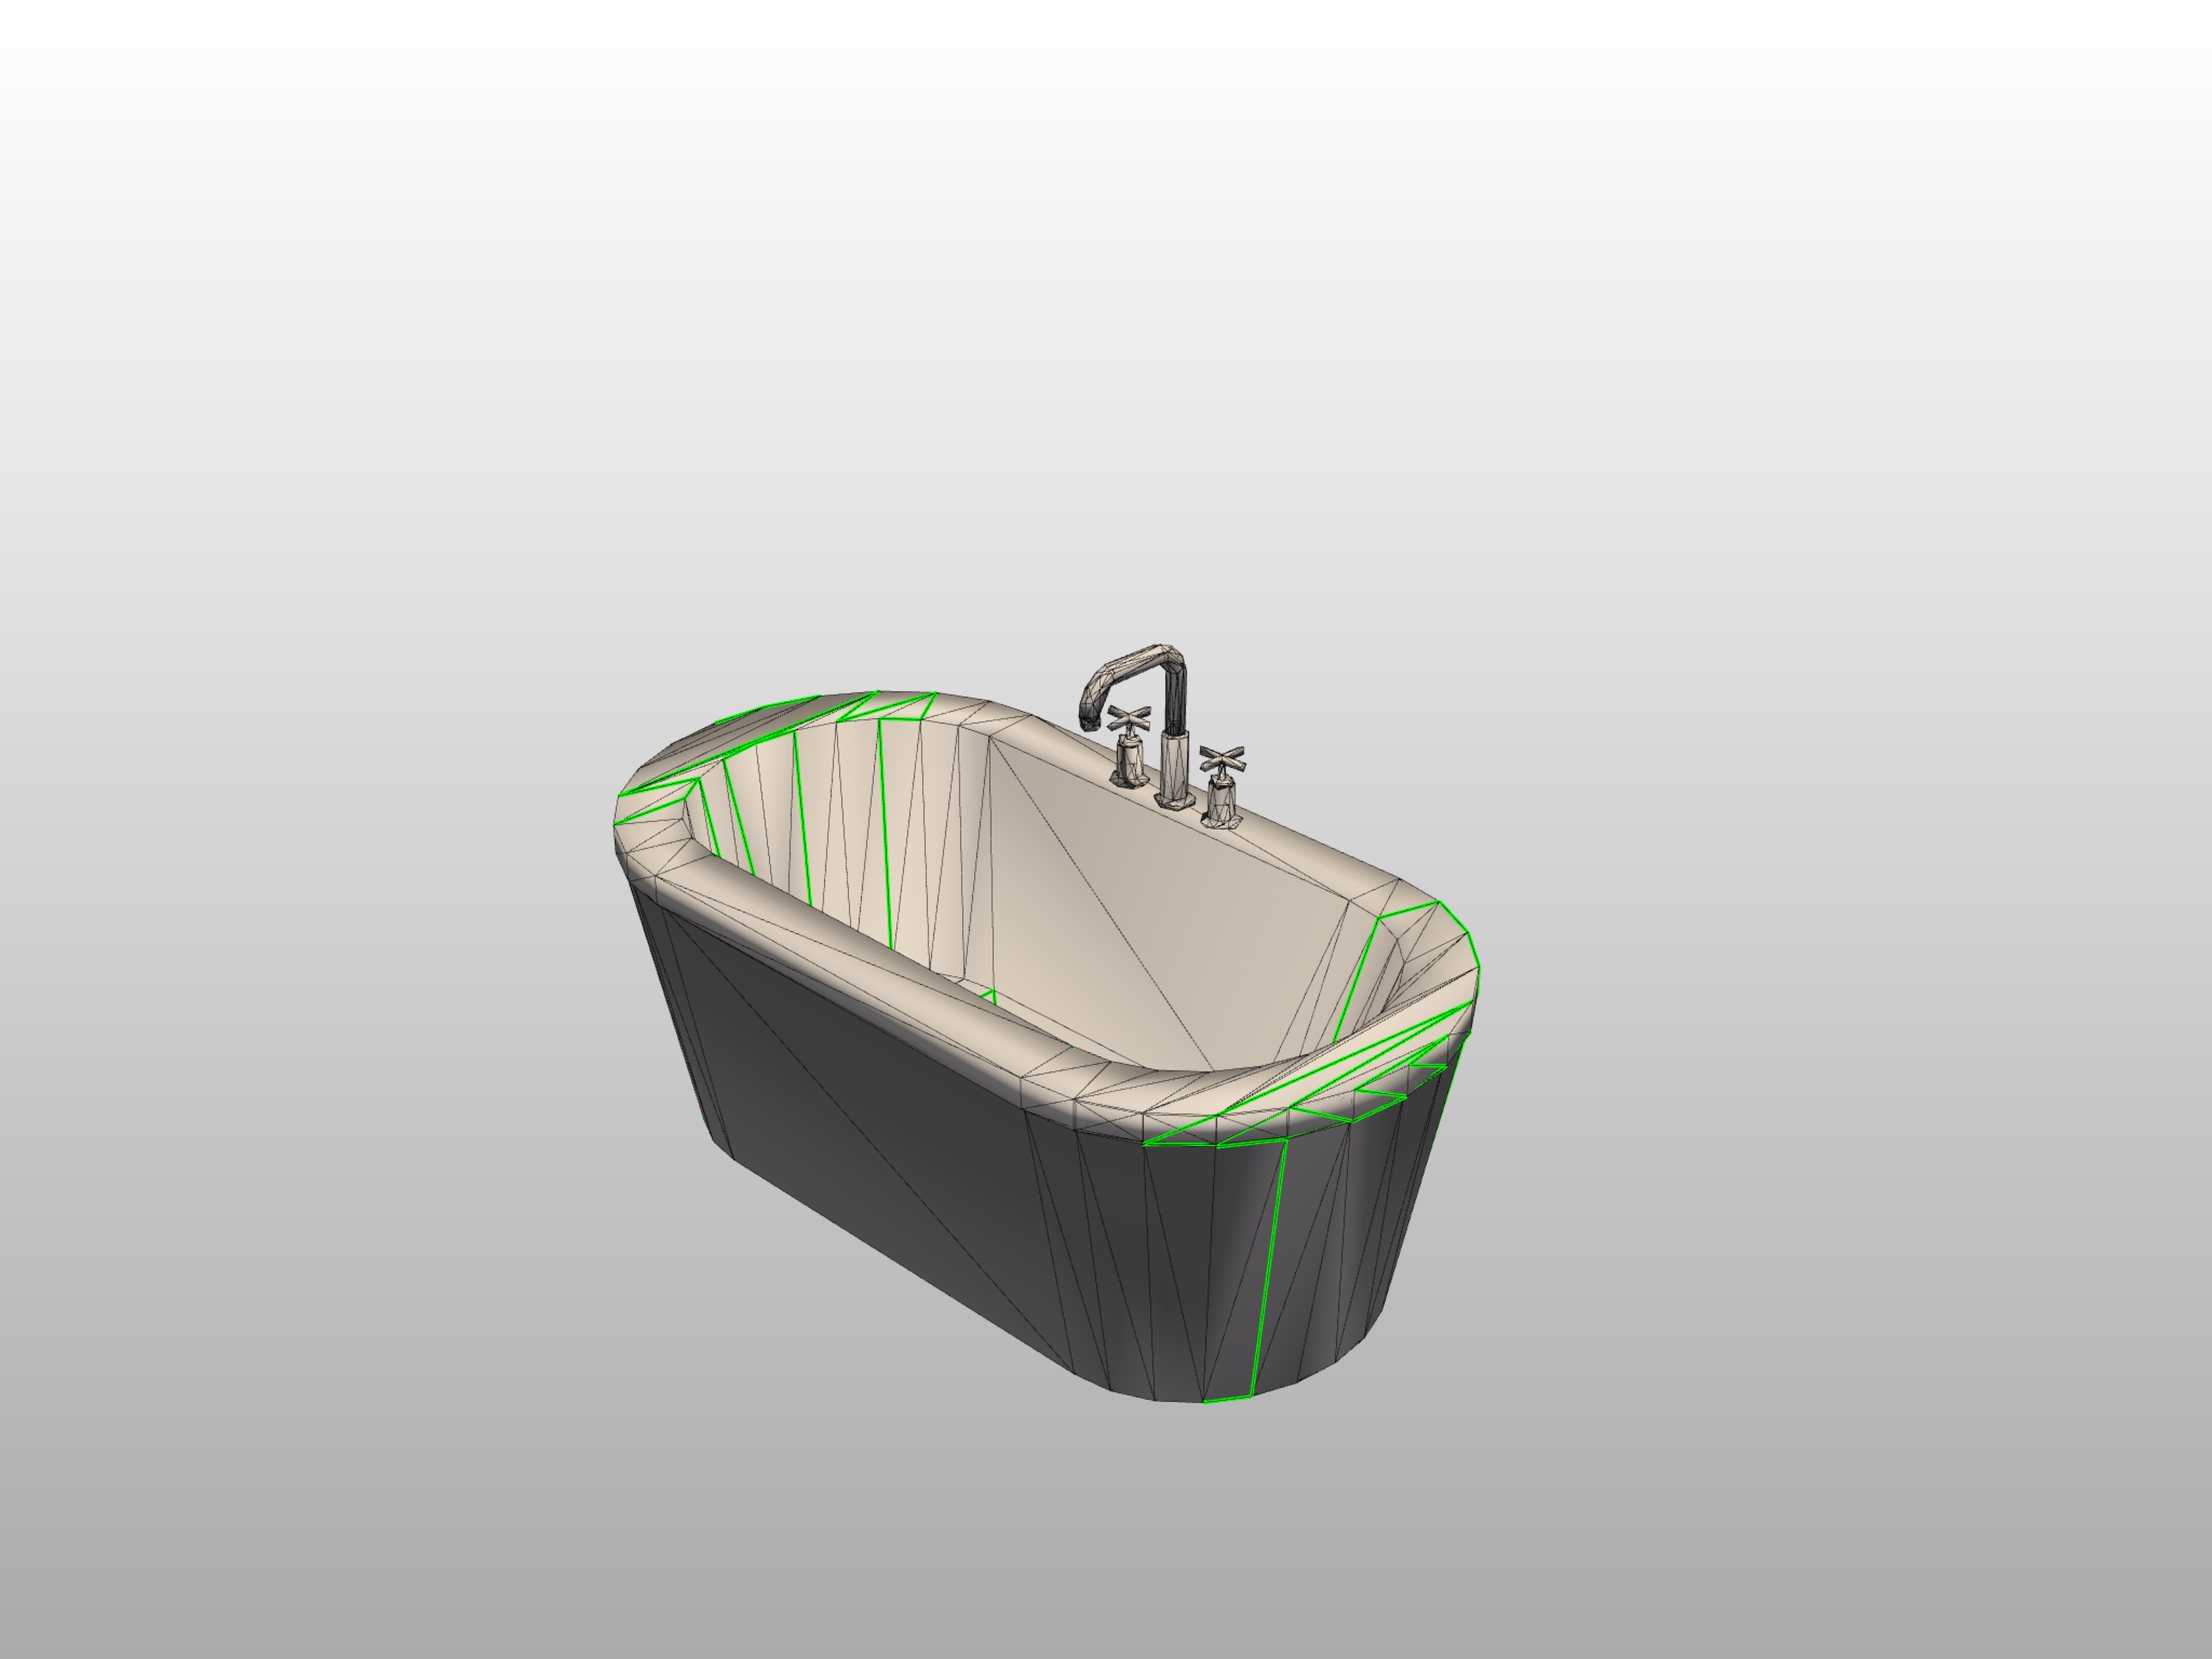}
  \caption{23\%}
\end{subfigure}%
\begin{subfigure}{.25\textwidth}
  \centering
  \includegraphics[width=.9\linewidth]{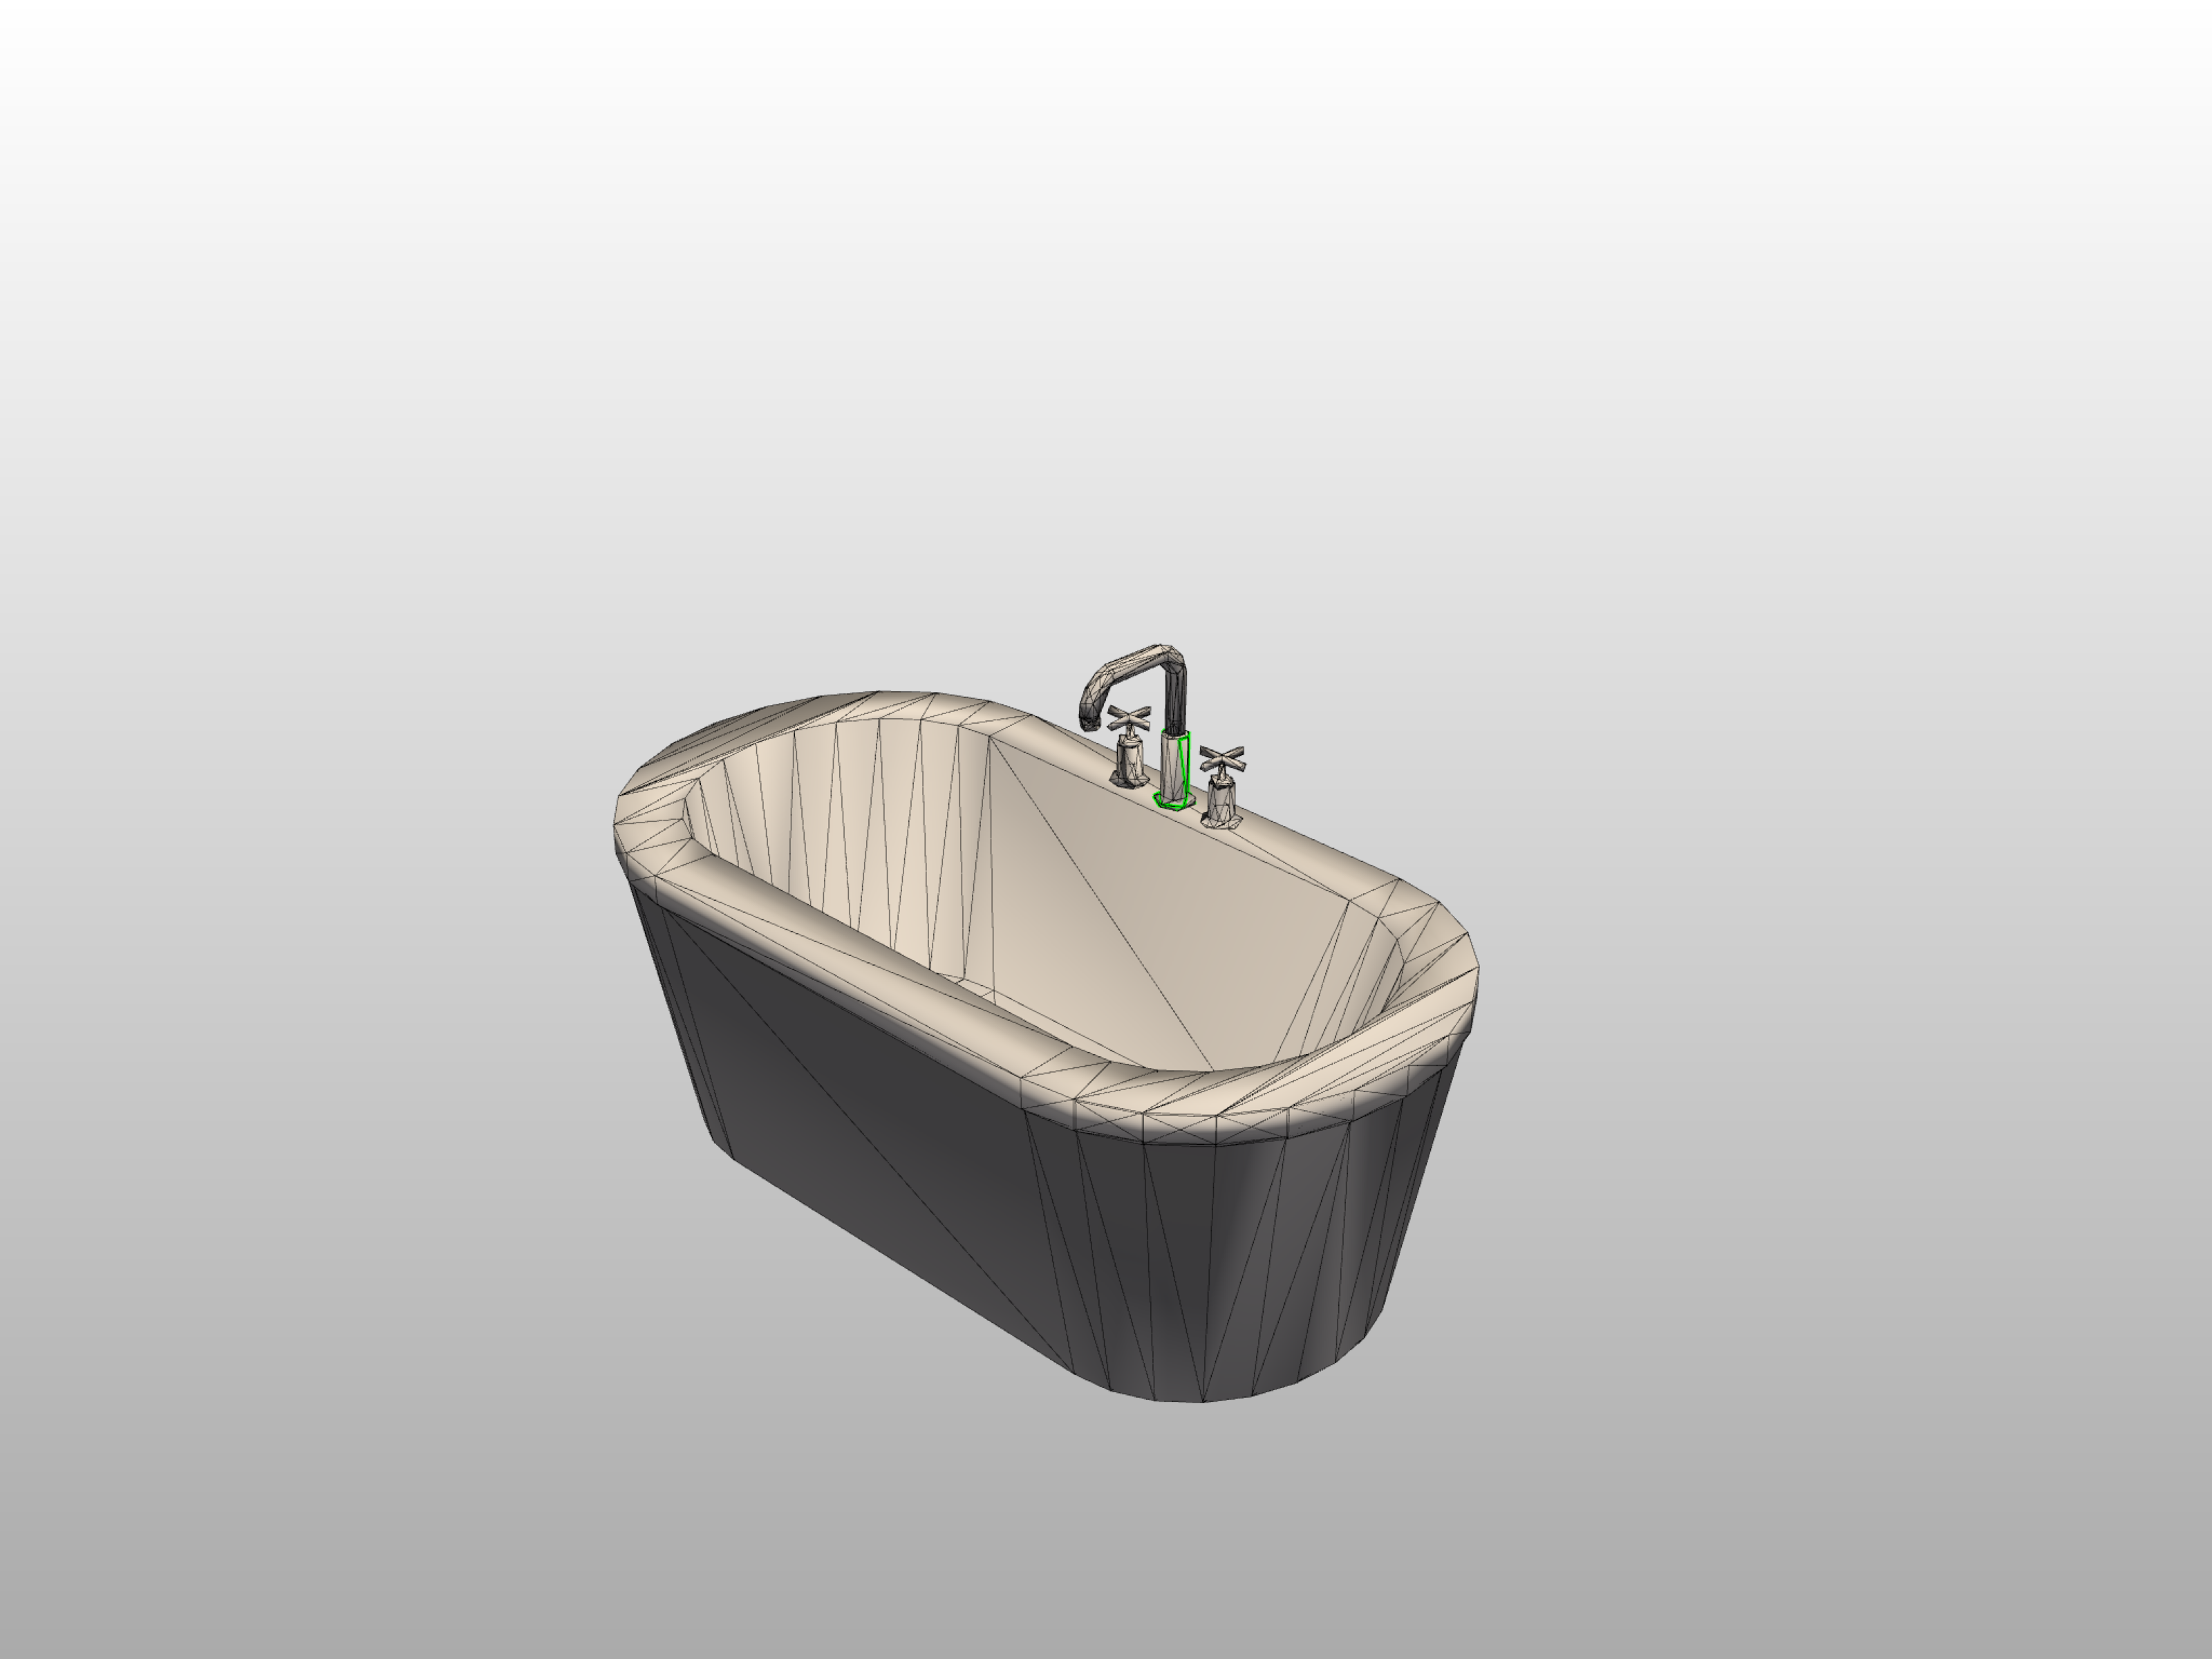}
  \caption{05\%}
\end{subfigure}%
\begin{subfigure}{.25\textwidth}
  \centering
  \includegraphics[width=.9\linewidth]{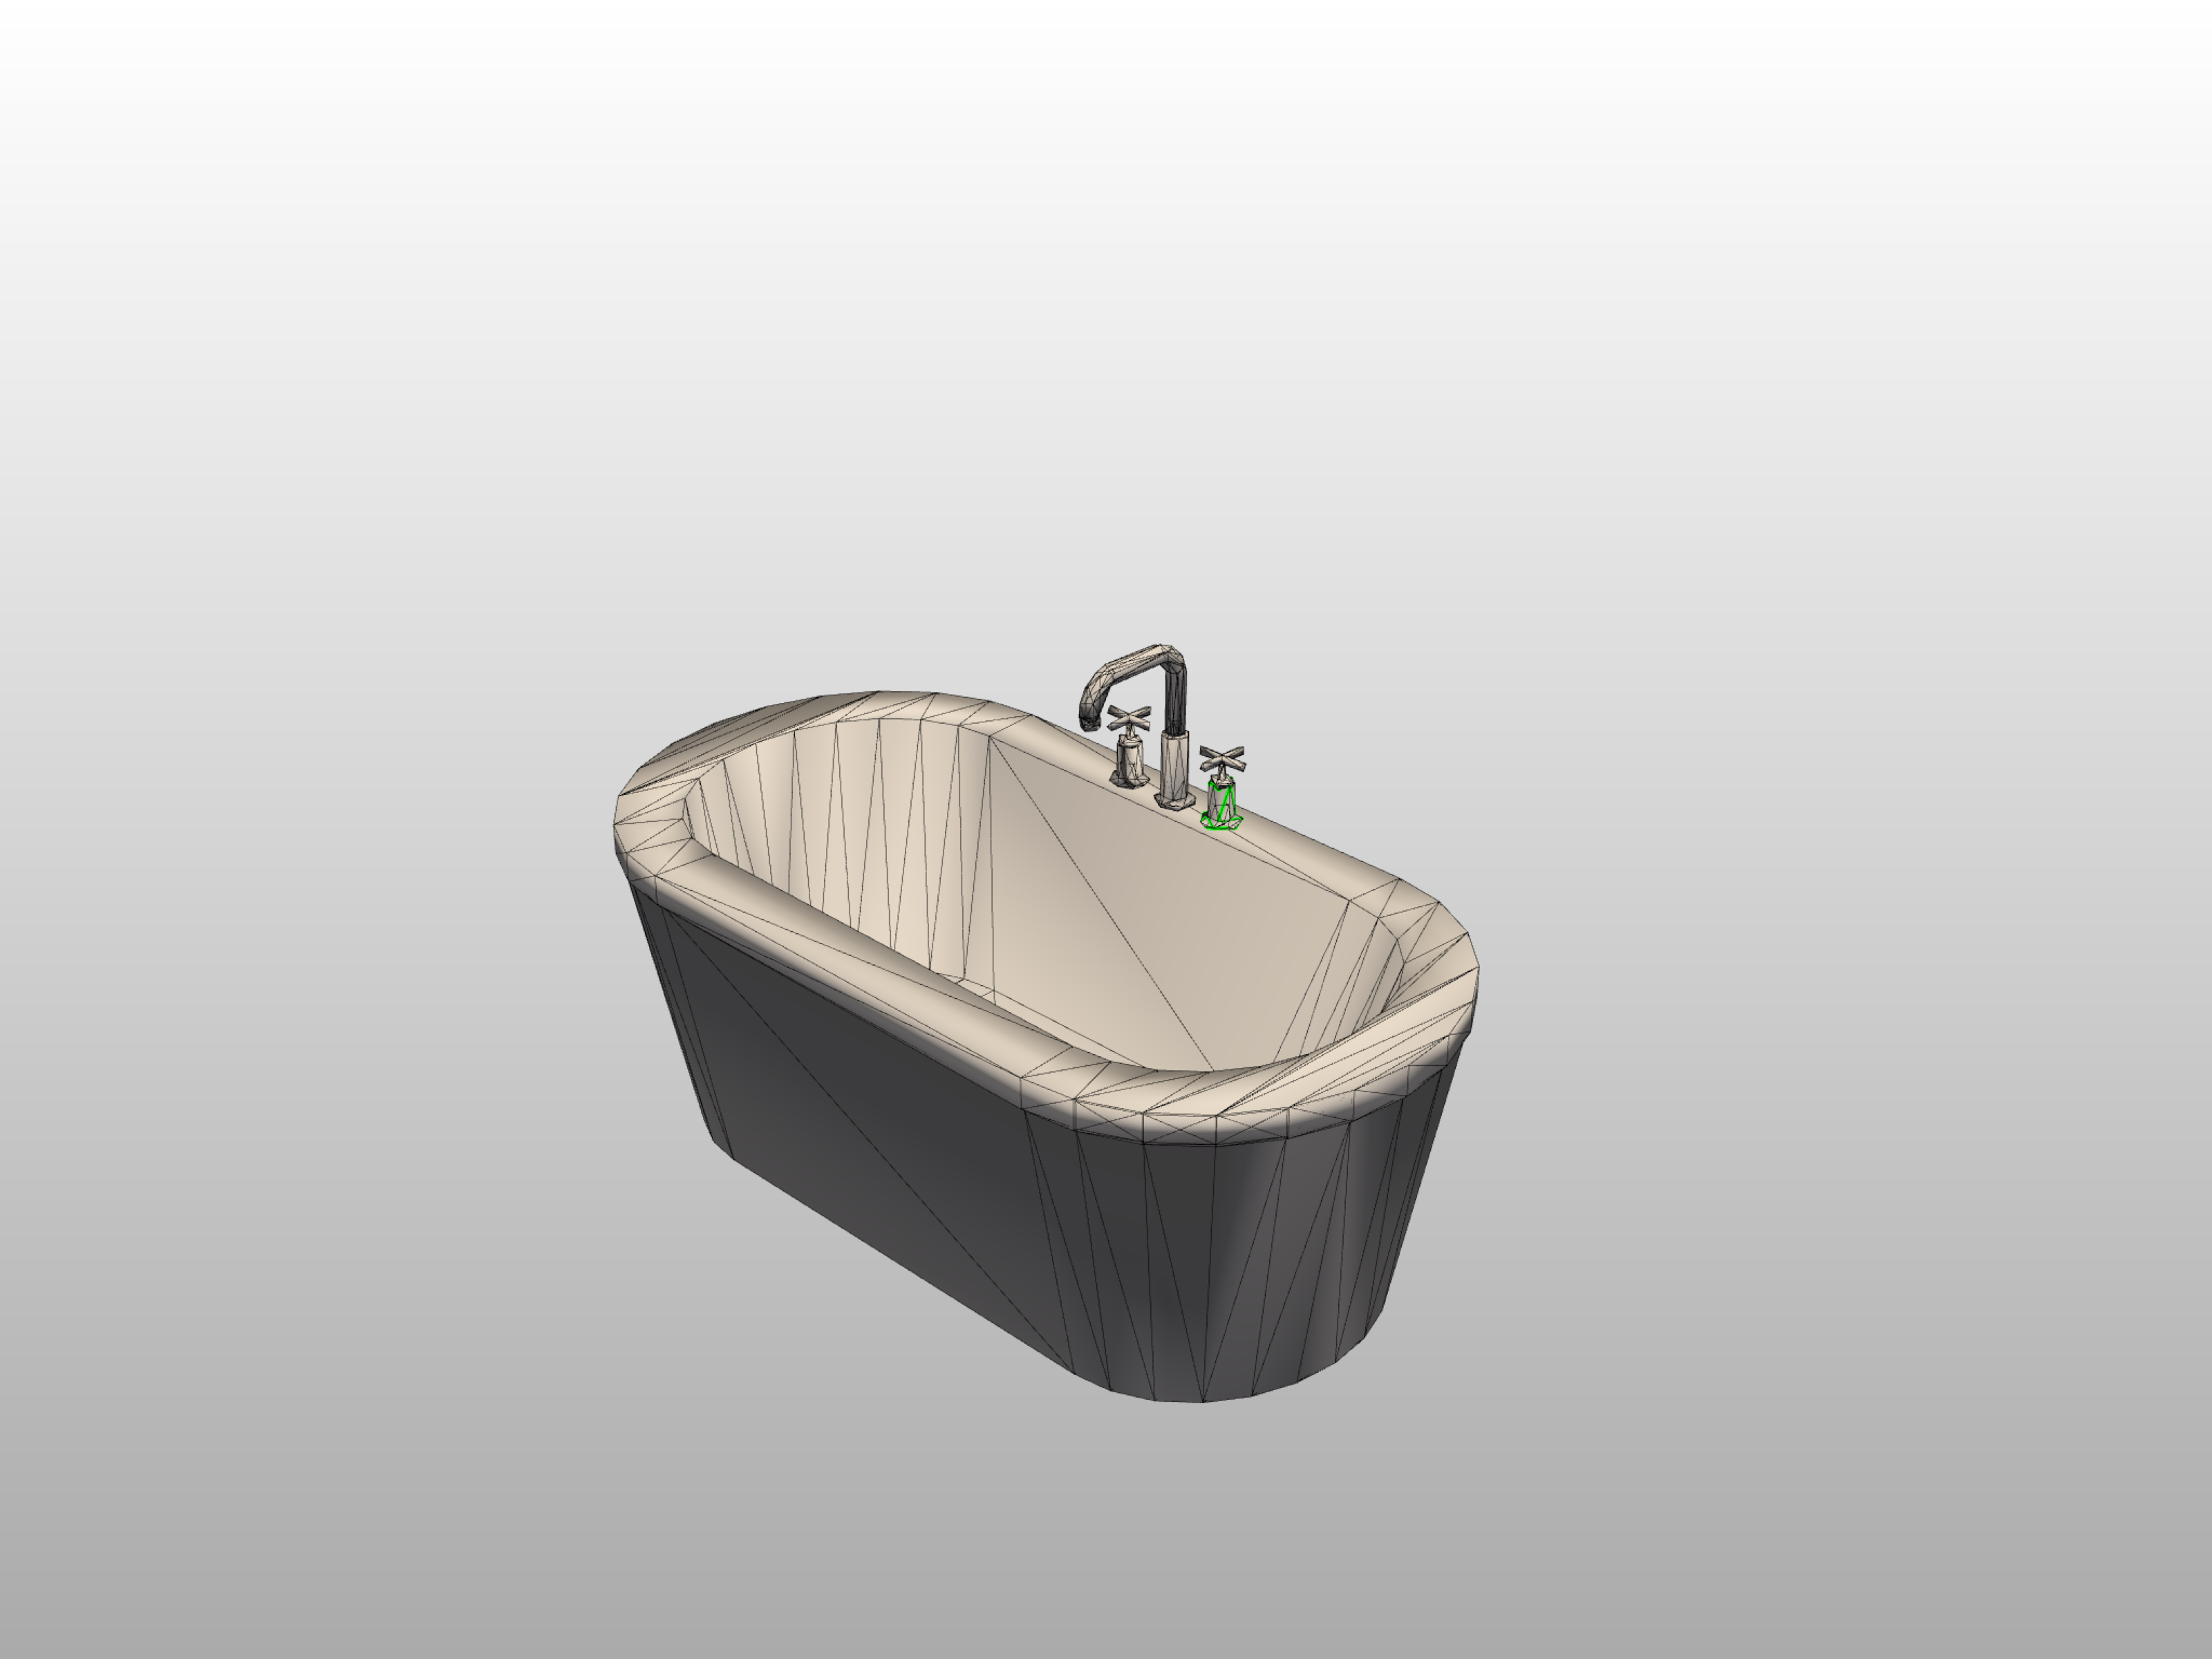}
  \caption{05\%}
\end{subfigure}%

\medskip
%  ==== second row ===== %
\begin{subfigure}{.25\textwidth}
  \centering
  \includegraphics[width=.9\linewidth]{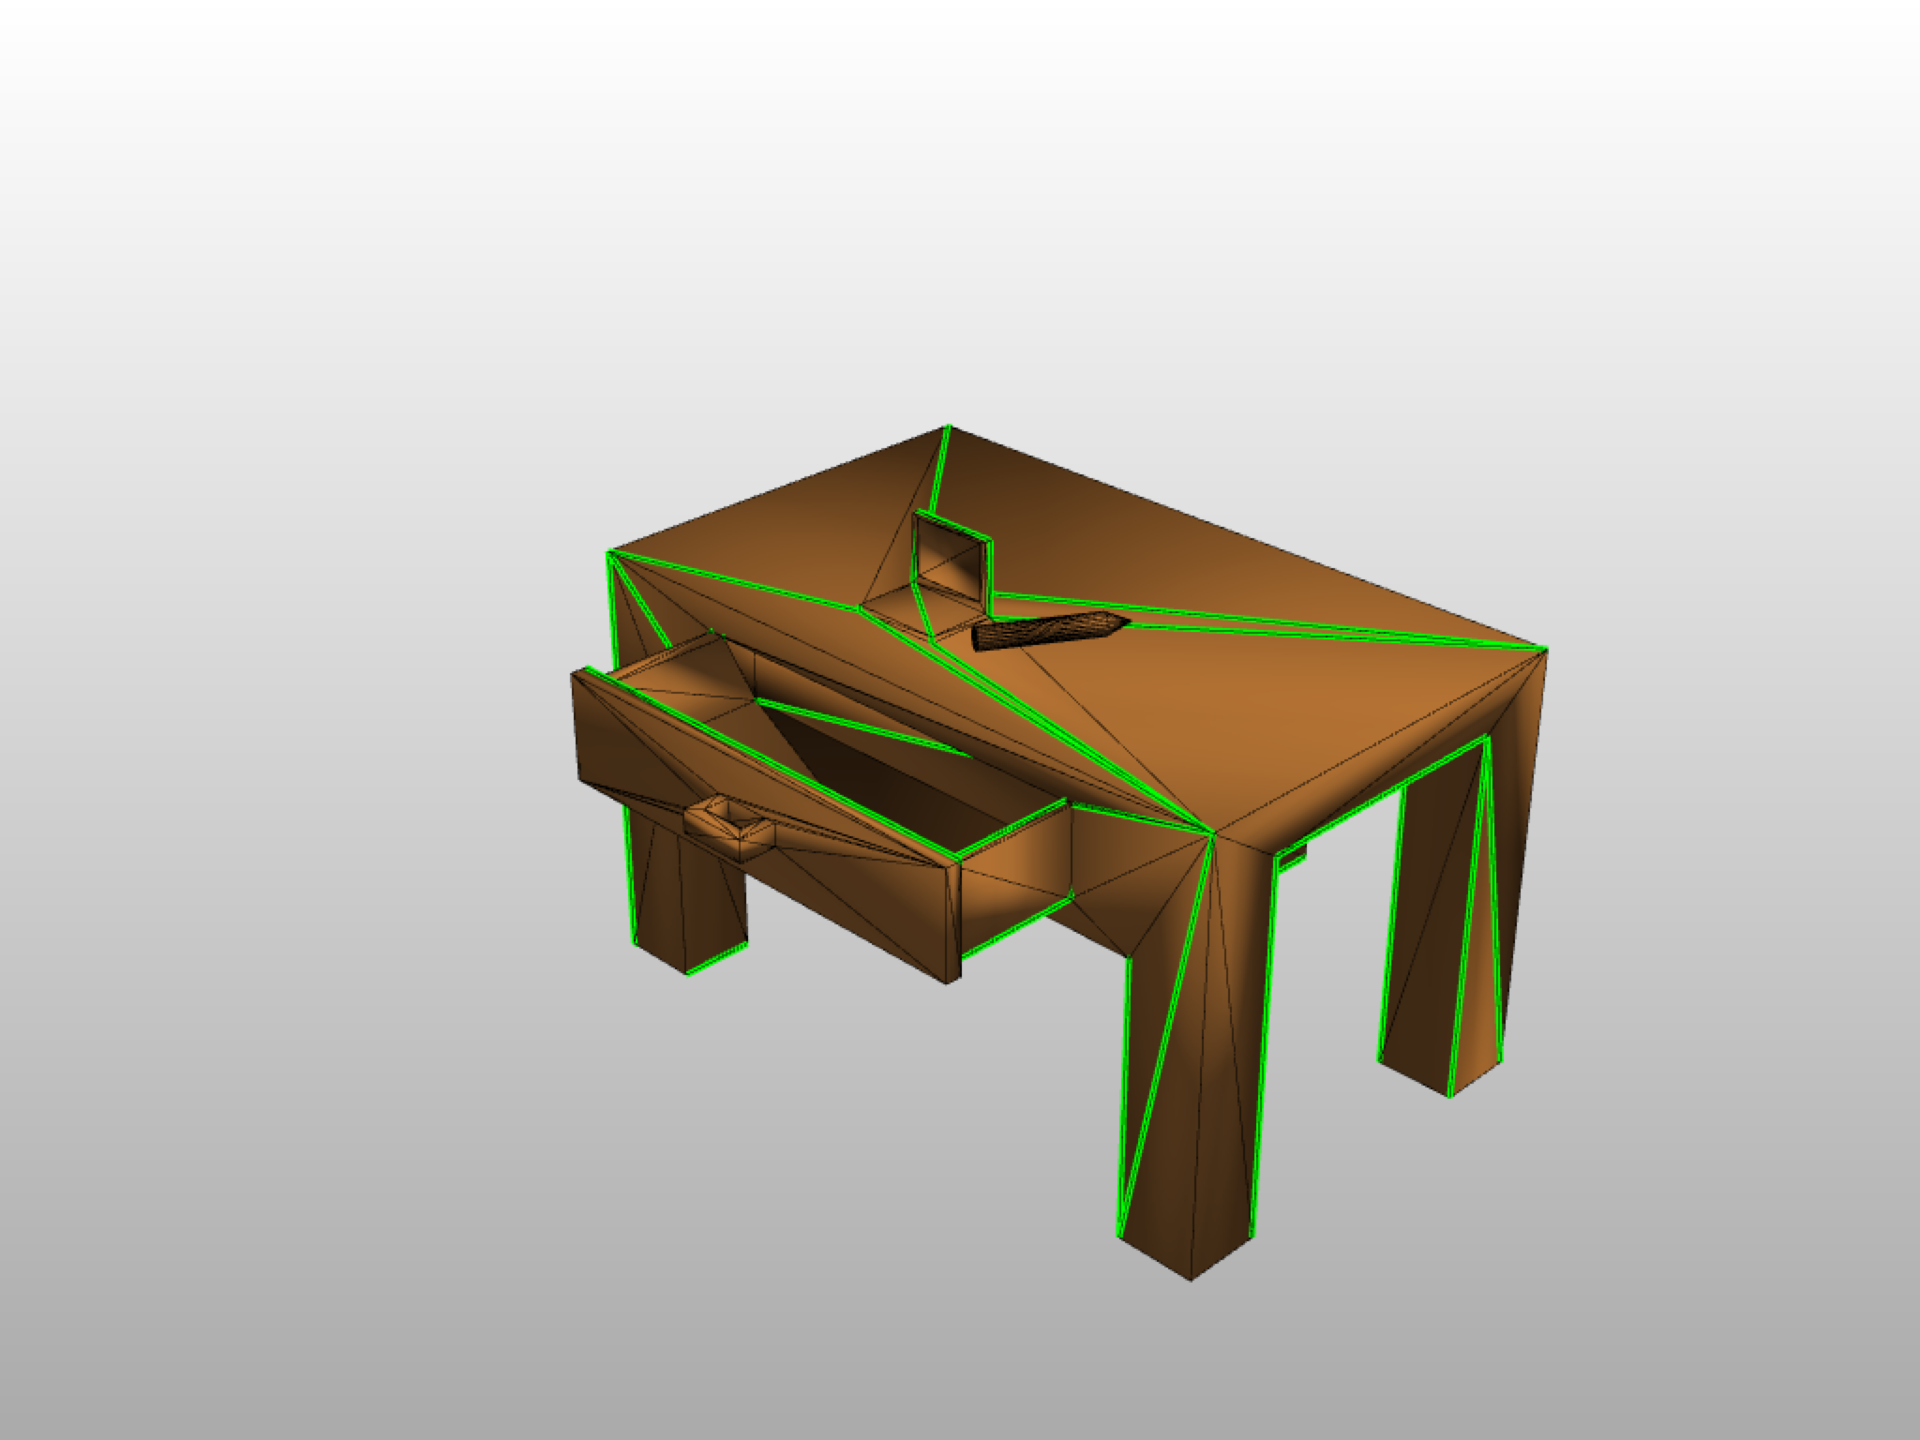}
  \caption{21\%}
\end{subfigure}%
\begin{subfigure}{.25\textwidth}
  \centering
  \includegraphics[width=.9\linewidth]{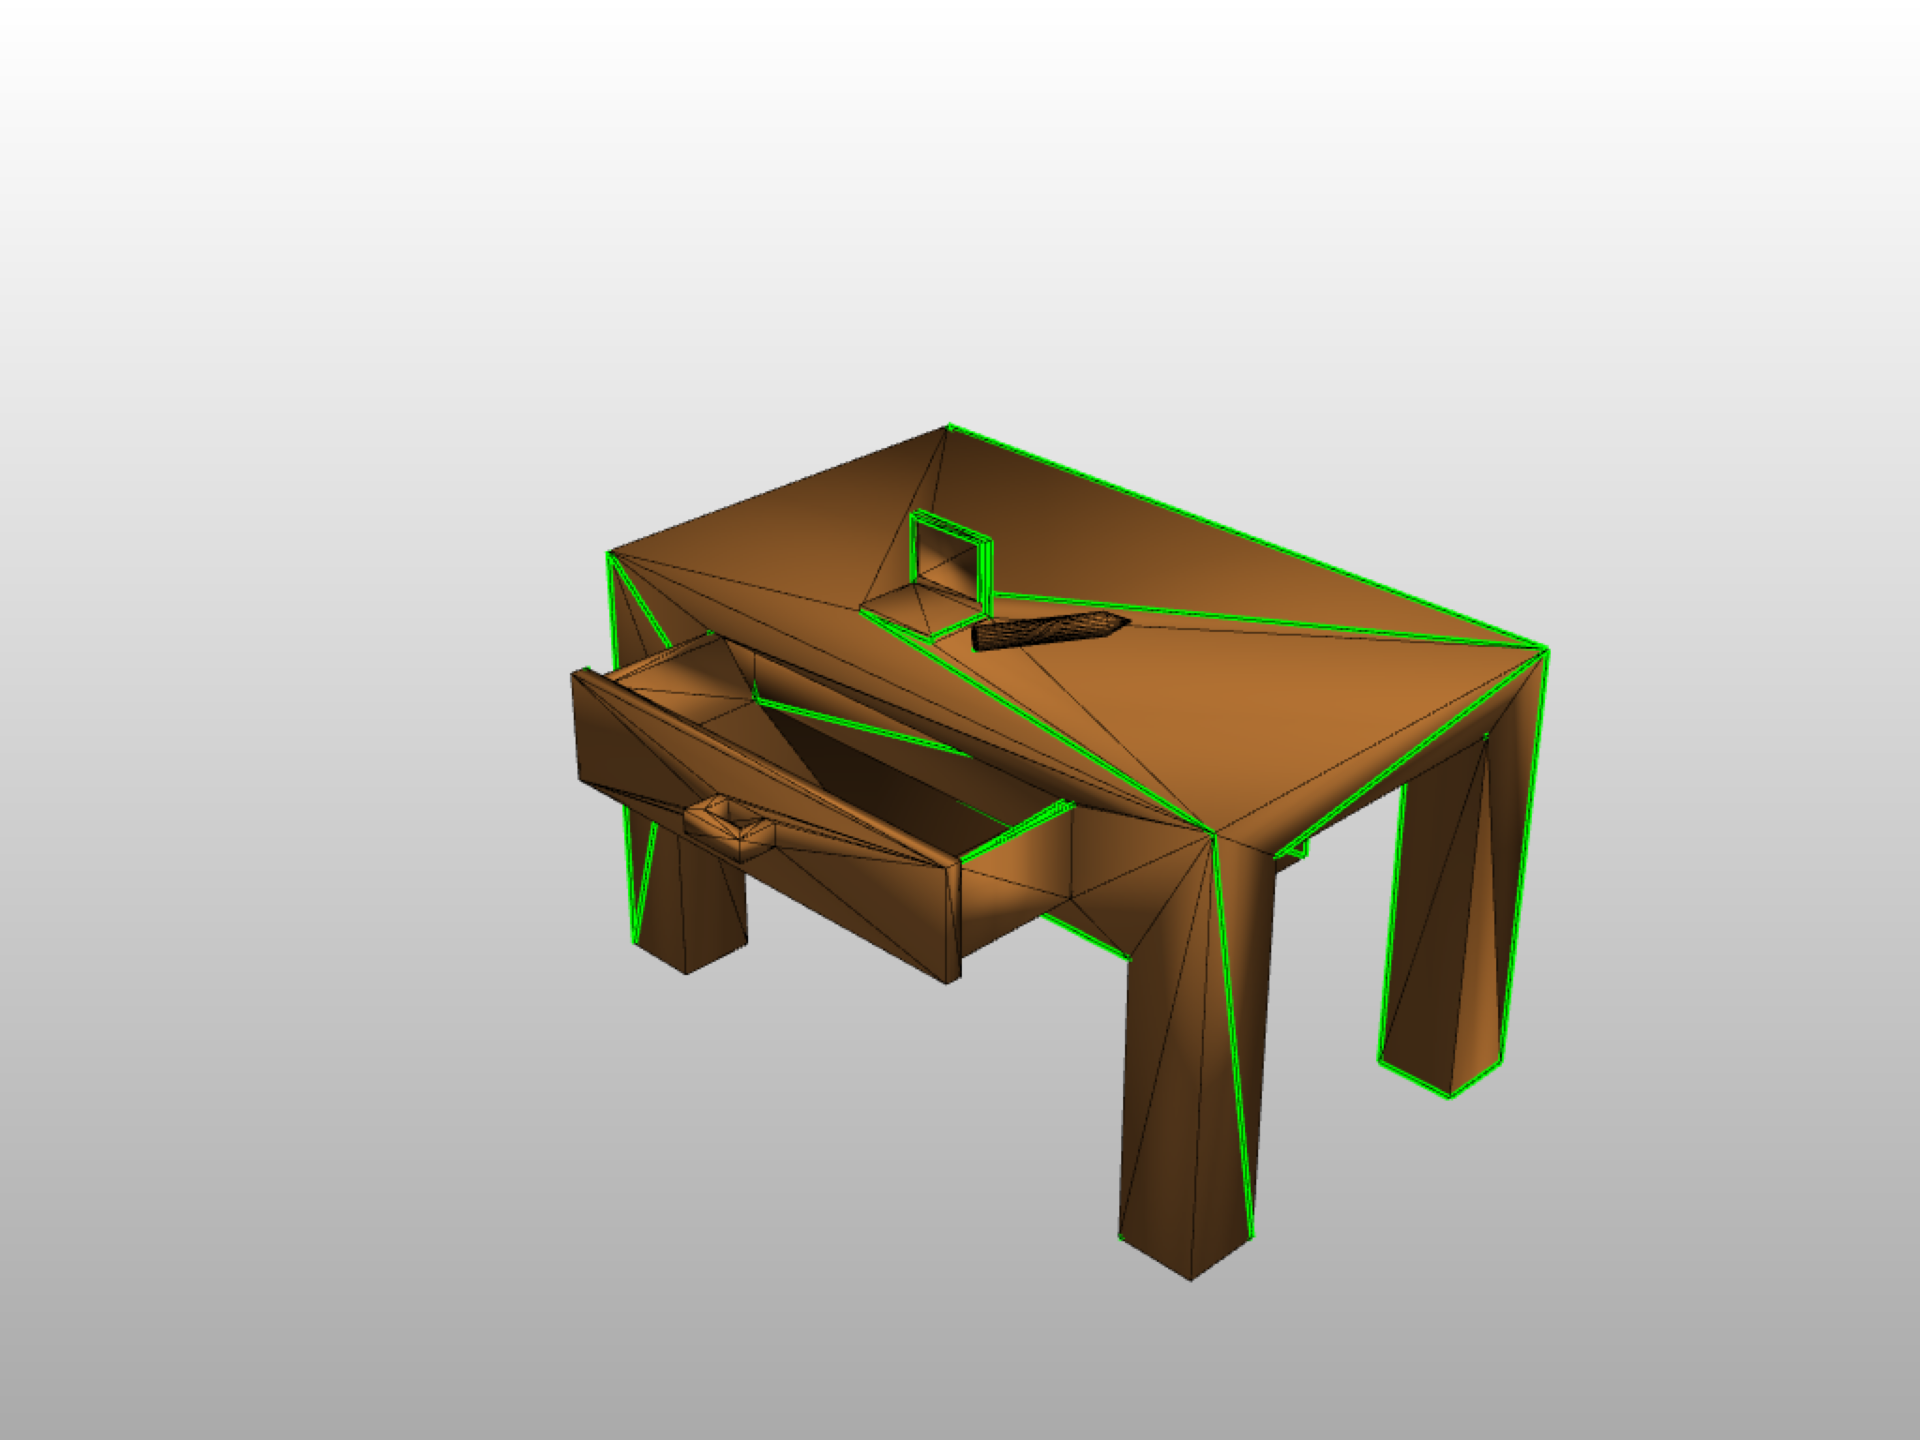}
  \caption{19\%}
\end{subfigure}%
\begin{subfigure}{.25\textwidth}
  \centering
  \includegraphics[width=.9\linewidth]{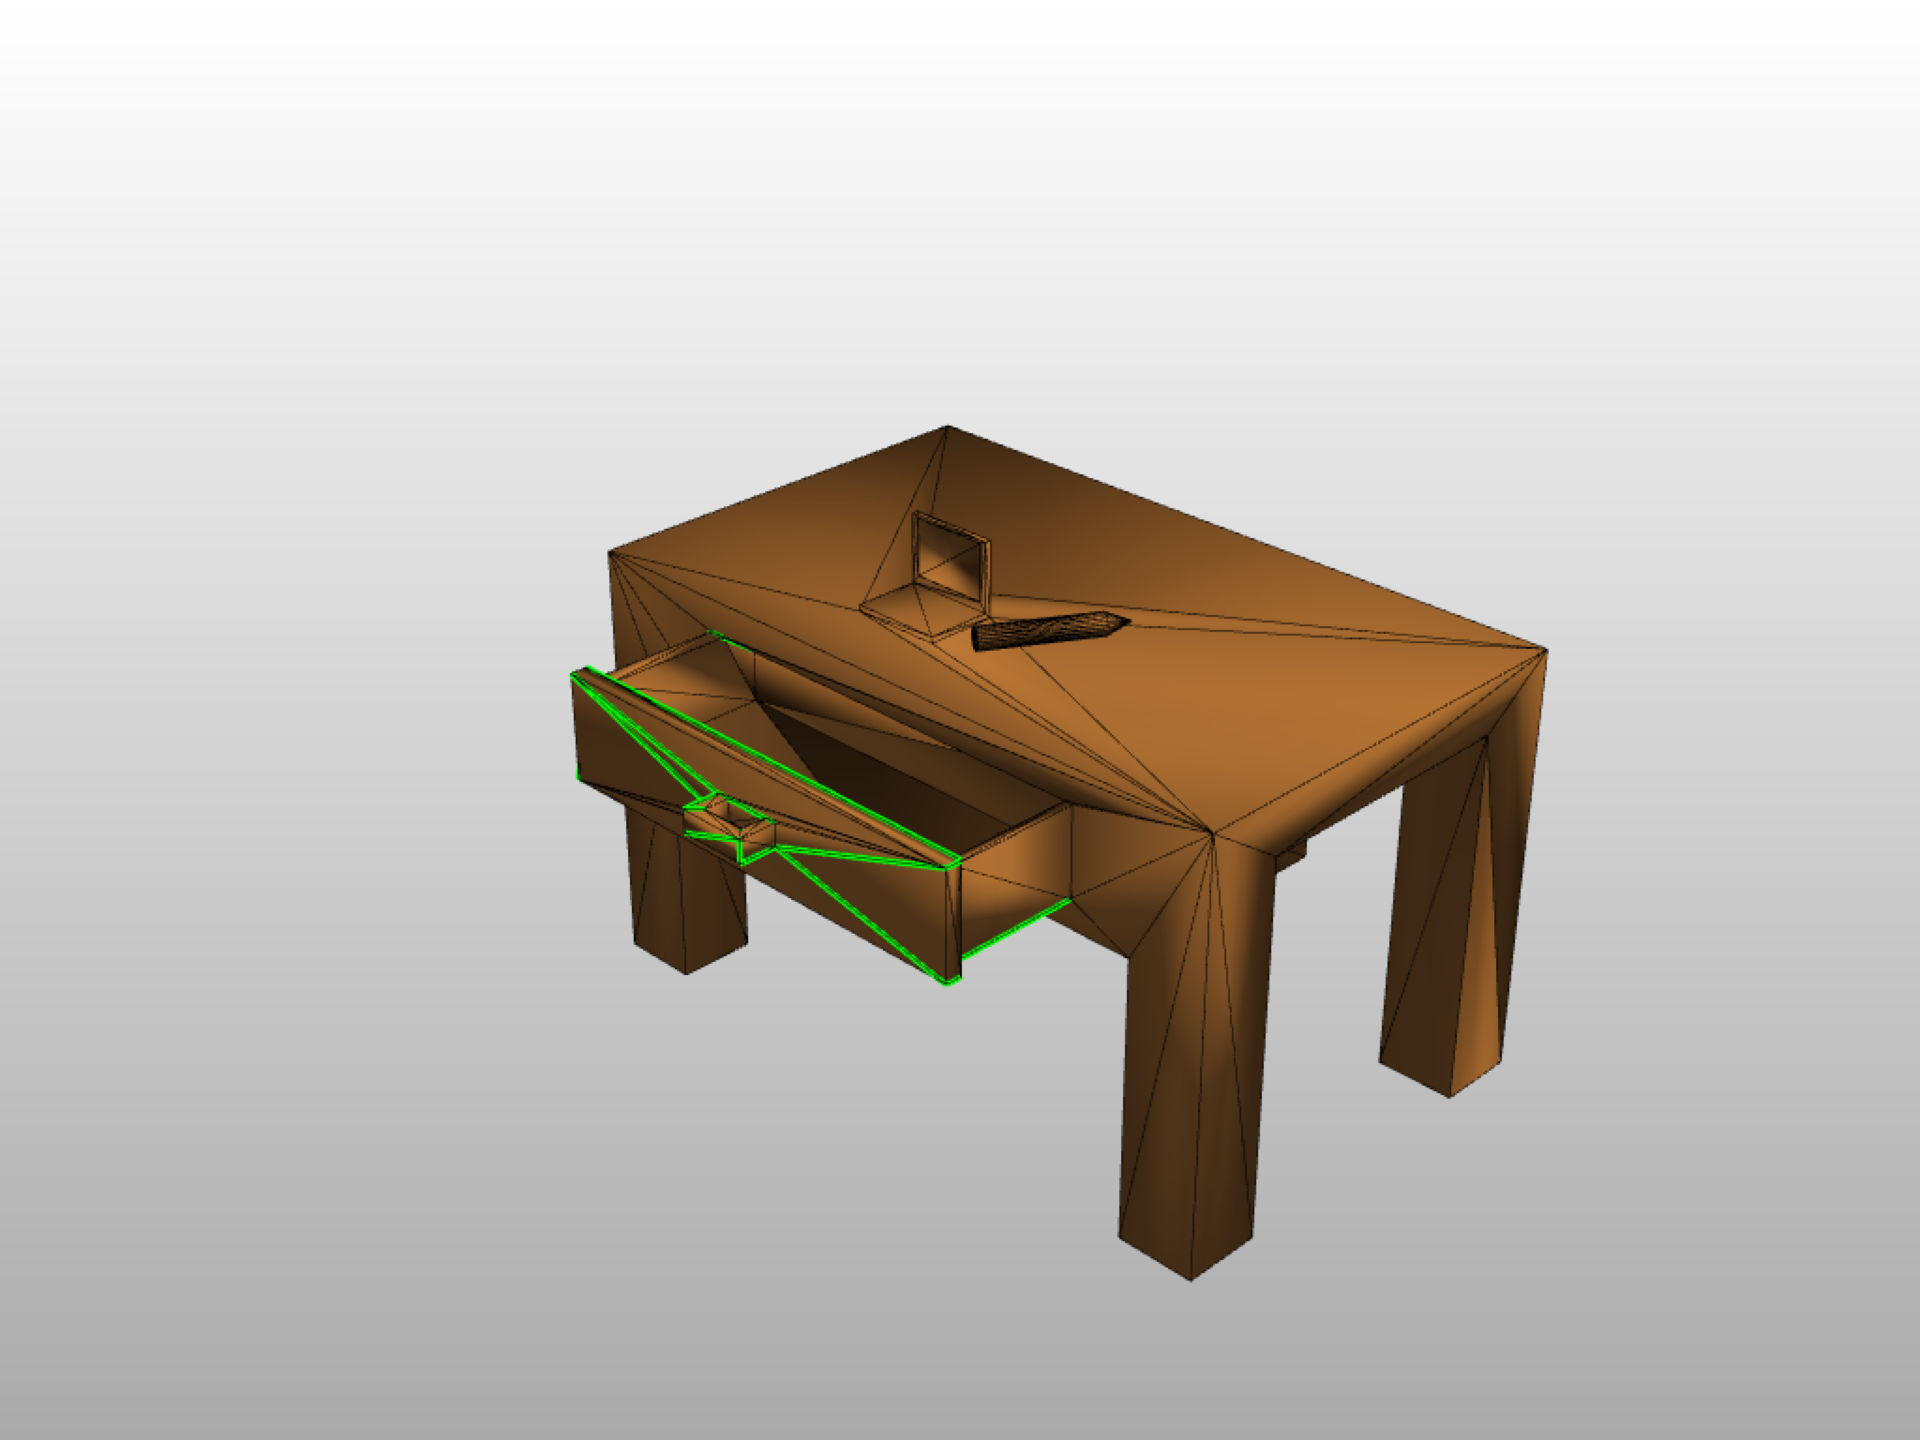}
  \caption{06\%}
\end{subfigure}%
\begin{subfigure}{.25\textwidth}
  \centering
  \includegraphics[width=.9\linewidth]{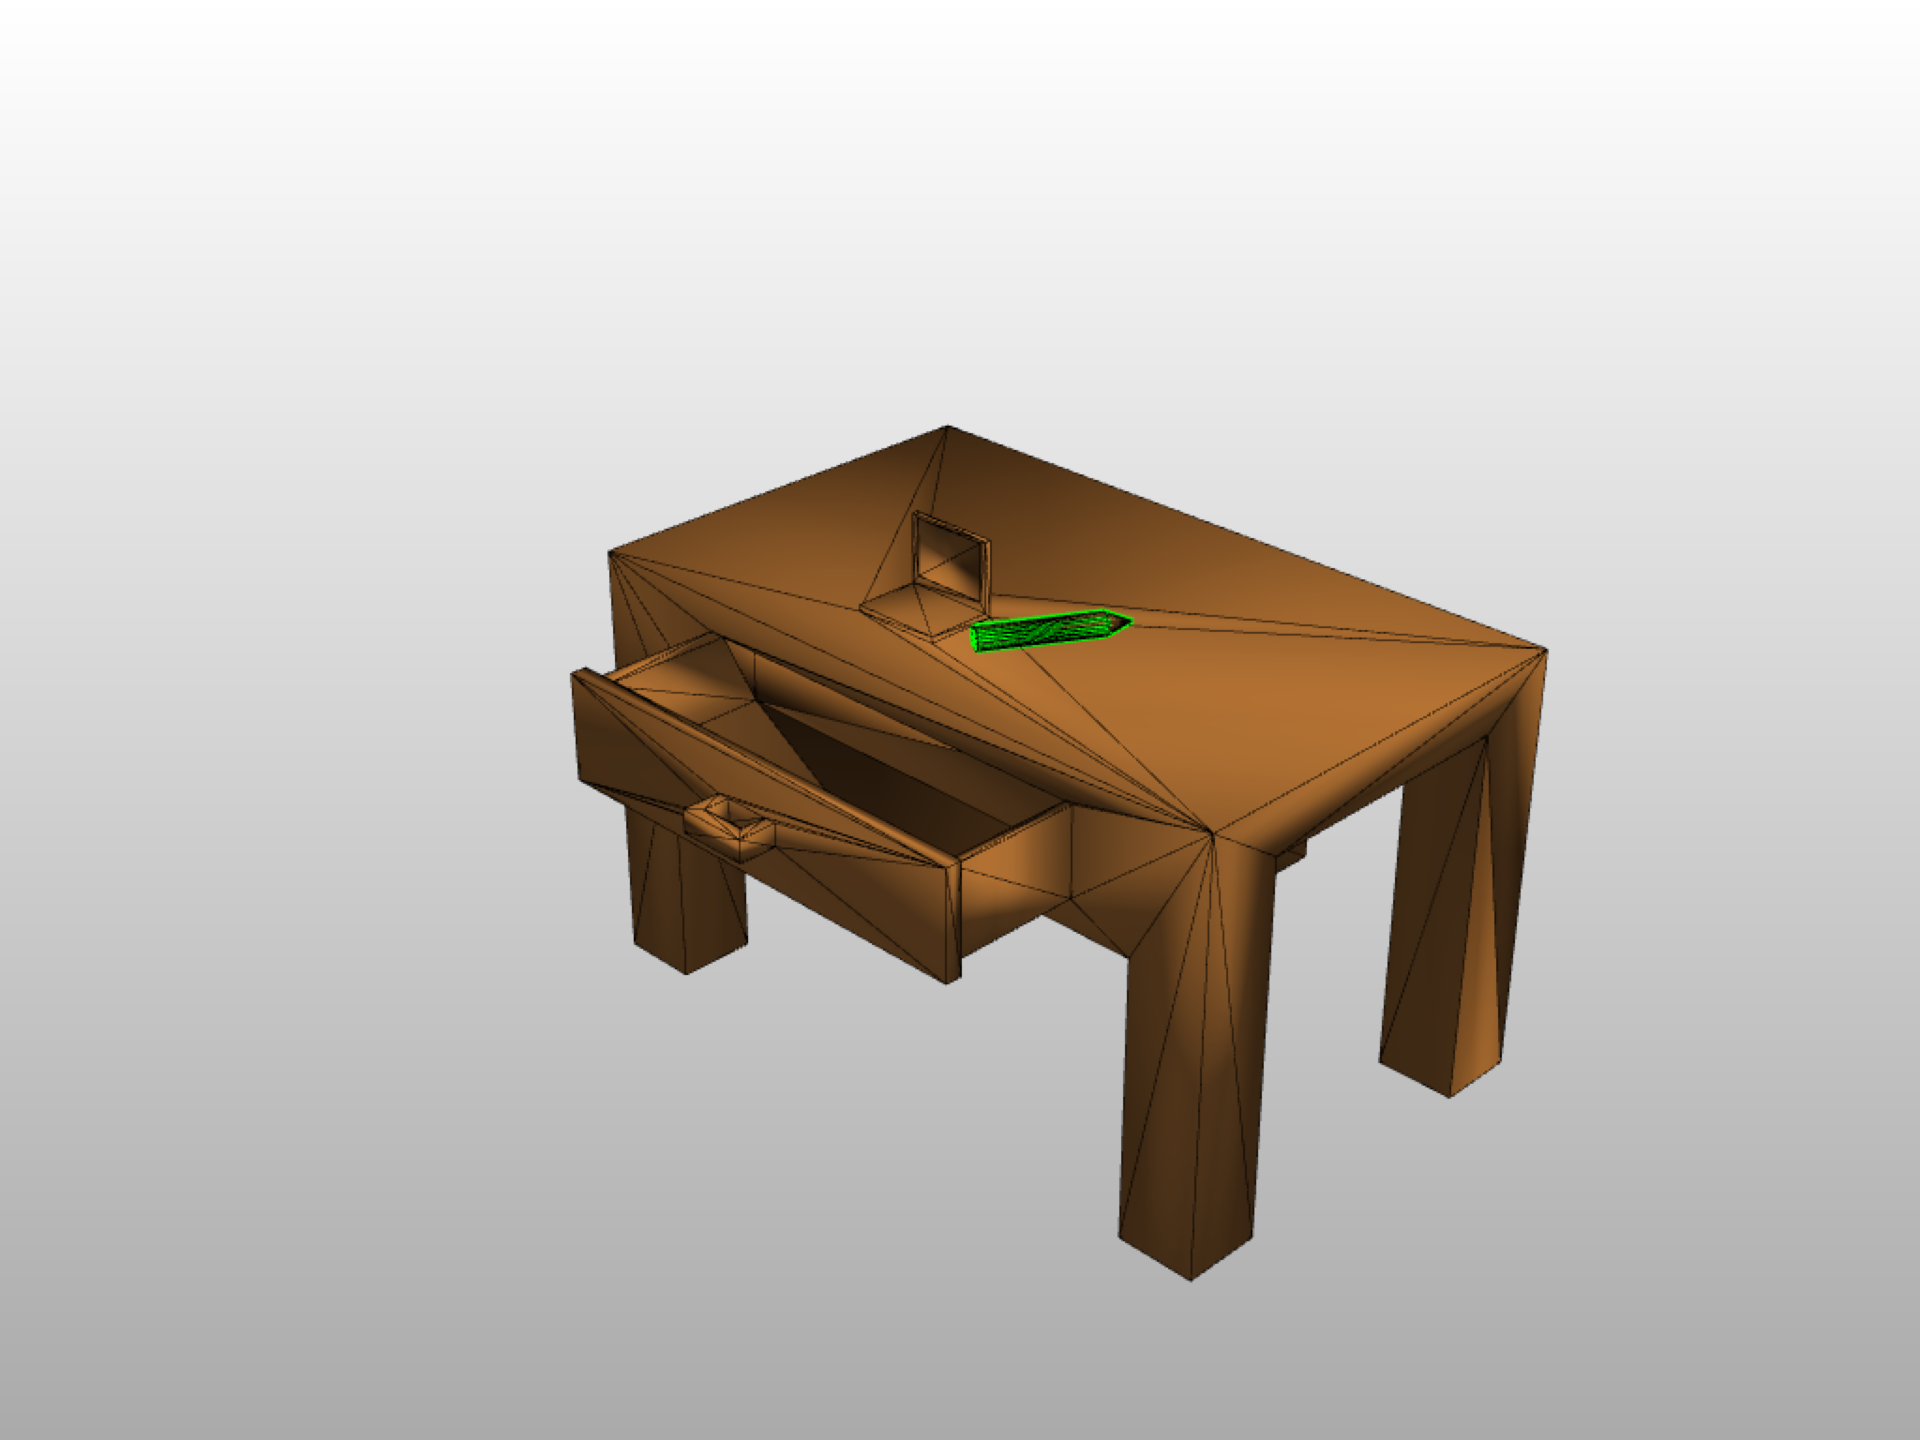}
  \caption{04\%}
\label{fig:AttentionCorrected}
\end{subfigure}
\caption{\ran{Two most attentive (left) and two least attentive (right) walks of a bathtub and a table. From averaging multiple walks the bathtub is classified as X, and the table as Y. We can see our model succeed in discarding information of walks with distracting details, as the pencil on table, or redundant details, as the bathtub tap (which can indicate sink class as well)}}
\end{figure*}

% ======== TO ADD - Time comparison!  (how much extra time in inference for 8 \ 64 walks, how much time saved by using 8 walks instead of 64. ============= %

\begin{tabular}{c c c c c c}
        \raisebox{0.5in}{most attended} &
        \includegraphics[height=.18\linewidth]{examples/ablation/corrected_alon_mn40/bathtub_rank_1_weight_14_cropped.png} &
   \\
        \raisebox{0.5in}{least attended} &
        \includegraphics[height=.18\linewidth]{examples/ablation/corrected_alon_mn40/sink_rank_8_weight_09_cropped.png} &
\end{tabular}

% =================== attended walks statistics for modelnet40 ============== %
% \begin{table}[h]
% \begin{center}
% \begin{tabular}{|c|c|c|c|c|}
% \hline
% Rank  & $1$ & $2$ & $7$ & $8$  \\
% \hline\hline
% Score &  $17.3 $ & $14.5 $  & $10.5 $ & $9.8 $  \\
% % W     &  $17.3 $ & $14.5$ & $13.1$ & $12.2$  & $11.6$ & $11.0$ & $10.5$ & $9.8$  \\
% Length &  $125$ & $119$ & $97$ & $92$  \\
% Coverage & 0.29611635& 0.30161918 &0.3054398 & 0.30905113& 0.30408236 & 0.30313935& 0.29586217 & 0.2836586 \\
% \hline
% \end{tabular}
% \end{center}
% \caption{\ran{\em{Attentive walks.} We present the average score, walk length and unique vertices visited for two most \& least attentive walks, averaged for ModelNet40 objects.
% }}
% \label{tab:stats}
% \end{table}
